# Supplementary material for: Massive MIMO-based Localization and Mapping Exploiting Phase Information of Multipath Components
Source: arXiv:1811.04494 source file (2019-06-12)
Supplement: Supplementary file 1 [file Appendix.tex]

\subsection{Interpolation of the measured beam pattern}
\label{Appendix_eadf}

The interpolated beam pattern matrix $ \B_{\text{A}} \in \mathbb{C}^{N_{\text{Rx}} \times N_{\text{a}}'N_{\text{e}}'} $ is formulated as
\begin{equation}
\B_{\text{A}} = [\B^{(\text{Rx})}(\varphi_{\text{s},i},\theta_{\text{s},i}) ],
\label{eq:Intepolated_BP_Matrix}
\end{equation}

where $ \B_{\text{A}} \in \mathbb{C}^{N_{\text{Rx}} \times N_{\text{a}}'N_{\text{e}}'} $ is a product of the effective aperture distribution function (EADF) \cite{Landmann_EADF_2004}, which performs efficient interpolation of the measured beam pattern via a discrete Fourier transform to obtain antenna responses of arbitrary azimuth and elevation angles that are off the sampling grid, where $ N_{\text{a}}' $ and $ N_{\text{e}}' $ denote the number of azimuth, elevation angular samples after interpolation.

\subsection{Noise Component Estimation}
\label{Appendix_noiseEst}
